# Supplementary material for: Sparse Weight Activation Training
Source: arXiv:2001.01969 source file (2020-10-31)
Supplement: Supplementary file 1 [file TopKProof.tex]

\section{Proof showing Top-K is the best sparsification function}\label{app:proof}

\textbf{Definition 1} Sparsifying Function ($f_{S}$): Given a parameter $1 < k \leq d$, let $f_{S}\colon \R^d \to \R^d$ be a function that selects 
k component of vector and sets the rest of the component to zero. For a vector $v\in \R^d, f_{S}(v) = \mathbb{I}_k(\vect{v})\odot\vect{v}$, where  $\mathbb{I}_k(\vect{v})$ is an indicator vector having k non-zero values determined by input vector $v$.

\textbf{Definition 2} Top-K Sparsifying Function ($f_{TOPK}$): Given a parameter $1 < k \leq d$, let $f_{TOPK}$ $\colon \R^d \to \R^d$ is a special sparsifying function that sets all but the k highest component of input vector in absolute value to zero. More precisely, for a vector $v\in \R^d$, $f_{TOPK}(v)=\mathbb{I}_{topk}(\vect{v})\odot\vect{v}$ where $\mathbb{I}_{topk}$ is an indicator function, $\mathbb{I}(i\in \{\pi_1,\cdots,\pi_k\})$, and $\pi$ is a permutation of $[d]$ such that $\abs{v}_{\pi_i} \geq \abs{v}_{\pi_{i+1}}$ for $i=1,\dots, d-1$.

\textbf{Definition 3} Sparsification Angle ($\theta$): For a vector $v\in \R^d$, the deviation in the direction caused by sparsification $f_{S}(.)$ is defined as the sparsification angle, i.e., it is the angle between the vector $v$ and sparse vector $f_{S}(v)$.

\begin{lemma} 
For any vector $v\in \R^d$ and of all the sparsifying function $f_{S}$, Top-K sparsifying function ($f_{TOPK}$) causes the minimum deviation in direction i.e. minimum sparsification angle.
\end{lemma}

\begin{proof}
Given a parameter $k\in[1,d]$, for a vector $\vect{v}=(v_1,\cdots,v_n)^{\rm T}\in\mathbb{R}^d$ let $\vect{f_{S}(v)}=(m_1 v_1,\cdots,m_d v_d)^{\rm T}\in \mathbb{R}^d$ such that $m_i\in \{0,1\} \ \forall i$, be the Top-K indicator mask i.e., $m_i=1$ only if $i^{th}$ component of $v$ is selected by the sparsifying function.

\begin{align}
\cos\langle f_{S}(\vect{v}), \vect{v}\rangle 
=\frac{f_{S}(\vect{v})\bm{\cdot} \vect{v}}{\|f_{S}(\vect{v})\|\|\vect{v}\|} 
=\frac{\sum\limits_{i=1}^d(m_i v_i^2)}{ \sqrt{\sum\limits_{i=1}^d(m_{i}v_{i})^2} \sqrt{\sum\limits_{i=1}^dv_{i}^2} } 
=\frac{\sum\limits_{i=1}^d(m_i v_i)^2}{ \sqrt{\sum\limits_{i=1}^d(m_{i}v_{i})^2} \sqrt{\sum\limits_{i=1}^dv_{i}^2} } \\
=\frac{\sqrt{\sum\limits_{i=1}^d(m_{i}v_{i})^2}}{\sqrt{\sum\limits_{i=1}^dv_{i}^2} }
=\frac{\|{f_{S}}(\vect{v})\|}{\|\vect{v}\|}
\end{align}
In other words,
\begin{align}
\text{Sparsifying Angle}(\theta) = \arccos \frac{\|{f_{S}}(\vect{v})\|}{\|\vect{v}\|}
\end{align}
$\arccos$ is a strictly decreasing function, so to minimize $\theta$, $\|{f_{S}}(\vect{v})\|$ must be maximized. Therefore Top-K component of the vector $v$ magnitude wise should be selected.  
\end{proof}
