# Supplementary material for: Sparse Weight Activation Training
Source: arXiv:2001.01969 source file (2020-10-31)
Supplement: Supplementary file 2 [file simulator.tex]

\subsection{Sparse Accelerator Speedup}
Sparse accelerators show significant performance and energy improvement even in the presence of irregular sparsity. 
To estimate the speedup on the sparse accelerator, we have used an architecture simulator for a recent sparse accelerator hardware proposal ~\cite{delmas2019bit}. 
The simulator only implements the forward pass, and therefore the simulator could not simulate the backward pass. However, the backward pass convolution is 
transposed convolution, which could be translated into standard convolution by simply rotating the input tensor~\cite{dumoulin2016guide}. 
So we estimated the backward pass speedup by transforming transpose convolution into standard convolution and using the inference simulator. 
Note, here the transformation overhead is not considered in the speedup. However, the overhead would be small in the actual hardware 
since transformation operation is a simple rotation operation, i.e., rotating the tensor along some axis and, therefore, could be implemented efficiently on hardware. 
\begin{table}[]
\caption{Speedup due to SWAT on ML Accelerator}
\label{tab:accelerator}
\centering
\begin{tabular}{@{}ccc@{}}
\toprule
Top-$K$ Sparsity & Forward Pass Speed Up & Backward Pass Speed Up \\ \midrule
0\%  & 1$\times$ & 1$\times$ \\
80\%  & 3.3$\times$ & 3.4$\times$ \\
90\%  & 5.6$\times$ & 6.3$\times$ \\ \bottomrule
\end{tabular}
\end{table}

The inference accelerator implements the forward pass and, therefore, speedup of the forward pass during training will be equal to the inference speedup.  
The computation in the backward pass is the deconvolution, also known as transposed convolution. 
The transposed convolution operation can be implemented using direct convolution~\cite{dumoulin2016guide}. 
%Therefore, to estimate the backward pass speedup, we mapped the backward pass on the inference accelerator and obtained the speedup. 
As shown in \autoref{tab:accelerator}, we can see that the SWAT algorithm accelerates training on average by $3.3\times$ and $5.9\times$ for $80\%$, and $90\%$ sparsity, respectively and the pruned model learned by SWAT will make the inference $3.3\times$ and $5.6\times$ faster at $80\%$, and $90\%$ sparsity respectively.
Thus, SWAT will be well suited for emerging sparse machine learning accelerator hardware designs.
